# Supplementary material for: Geometry Enhancements from Visual Content: Going Beyond Ground Truth
Source: arXiv:2012.08248 source file (2022-03-05)
Supplement: Supplementary file 1 [file 6.supplementary.tex]

\clearpage
\appendix
\section*{supplementary}

% \subsection*{Failed cases}
% \begin{figure}[!htb]
%     \includegraphics[width=0.5\textwidth]{images/FailDIML2.jpg}
%     \caption{Failure example: Image taken from \cite{DIML}, the text appears in the predicted depth as causing depth changes. This is caused by the strong gradients in the RGB image that the letters create.}
% \label{fig:Fail}
% \end{figure}

% Our network often fails over paintings and writings that cause string edges in the RGB images and does not effect depth.
% For dealing with these failed cases we can research the following approach: First, training a different network that segments painting, text, and other strong misleading gradients. Then, we can block them in the RGB image, preventing the gradients from reaching the network.

\subsection*{Hyperparameter tuning}

The hyperparameters of the networks, specifically the weights of the different loss functions were chosen manually.
The ratio between the unweighted losses differs between data-sets. Hence, we first run several batches where all weights are set to 1. Second, we normalize the losses, each loss according to it's mean. Third, we weight the normalized losses such that the sleeve loss is set to 1, the sleeve loss is set to 0.5, and the others are set to 0.1. 
After several epochs of training, we can tweak these losses according to the visual results.

% Ablation table:

% \begin{center}
% \centering
% \begin{table*}
%  \begin{tabular}{p{0.15\linewidth}|p{0.115\linewidth}p{0.115\linewidth}p{0.115\linewidth}p{0.115\linewidth}p{0.115\linewidth}p{0.115\linewidth}}

%  \toprule
%  & MSE & rMSE & MAE & ABS REL & PSNR & Median Err. \\ [1.0ex] 
% \toprule
%  Sleeve loss & 0.364 & 0.376 & 0.250 & 0.078 & 35.80 & 0.254 \\ [1ex]

%  False Edge loss & \textbf{0.193} & 0.293 & 0.228 & 0.075 & 37.985 & 0.239 \\ [1ex]

%  Total Variation & 0.379 & 0.353 & 0.246 & 0.065 & 38.985 & 0.065 \\ [1ex]
 
%  Cycle loss & 6.248 & 1.797 & 1.556 & 0.572 & 4.351 & 4.645 \\ [1ex]
% \midrule
%  Full Architecture & 0.196 & \textbf{0.280} & \textbf{0.172} & \textbf{0.054} & \textbf{39.903} & \textbf{0.05} \\ [1ex]
%  \bottomrule

% \end{tabular}
%   \caption{Numerical results for ablation study. Each line represents the results of the network with a different part missing.}
% \label{fig:Ablation2}
% \end{table*}
% \end{center}
